# Supplementary material for: Learnable Permutation for Structured Sparsity on Transformer Models
Source: arXiv:2601.22980 source file (2026-01-30)
Supplement: Supplementary file 1 [file appendix.tex]

%\section{Supplementary Material}

\subsection{Channel Permutation for Transformer Layers}

Applying channel permutations in Transformer architectures is challenging due to the structural coupling within multi-head self-attention (MHA) and feed-forward networks (FFN). Unlike sequential linear layers, Transformer blocks use parallel projections that share inputs and have interdependent weights, requiring coordinated, structure-aware permutations.

In the MHA module, the input \(\mathbf{X} \in \mathbb{R}^{B \times T \times d_{\text{hidden}}}\) is linearly projected into query, key, and value tensors using \(\mathbf{W}^{\top}_\mathrm{q}, \mathbf{W}^{\top}_\mathrm{k}, \mathbf{W}^{\top}_\mathrm{v} \in \mathbb{R}^{d_{\text{hidden}} \times d_{\text{hidden}}}\). These are used for attention computation, producing \(\mathbf{X}_\text{Attn} \in \mathbb{R}^{B \times T \times d_{\text{hidden}}}\), which is then projected by \(\mathbf{W}^{\top}_\mathrm{o} \in \mathbb{R}^{d_{\text{hidden}} \times d_{\text{hidden}}}\). Due to input sharing, a channel permutation matrix \(\mathbf{P}_{\text{in}} \in \mathbb{R}^{d_{\text{hidden}} \times d_{\text{hidden}}}\) applied to \(\mathbf{W}^{\top}_\mathrm{o}\) must also be consistently applied to the output channels of \(\mathbf{W}^{\top}_\mathrm{q}, \mathbf{W}^{\top}_\mathrm{k}, \mathbf{W}^{\top}_\mathrm{v}\).

\begin{equation}
\begin{aligned}
\widehat{\mathbf{W}}^{\top}_\mathrm{q} = \mathbf{W}^{\top}_\mathrm{q} \mathbf{P}^{\top}_{\text{in}}, \quad
\widehat{\mathbf{W}}^{\top}_\mathrm{k} = \mathbf{W}^{\top}_\mathrm{k} \mathbf{P}^{\top}_{\text{in}}, \\
\widehat{\mathbf{W}}^{\top}_\mathrm{v} = \mathbf{W}^{\top}_\mathrm{v} \mathbf{P}^{\top}_{\text{in}}, \quad
\widehat{\mathbf{W}}^{\top}_\mathrm{o} = \mathbf{P}_{\text{in}} \mathbf{W}^{\top}_\mathrm{o}.
\end{aligned}
\label{eq:3}
\end{equation}

Given the standard attention computation formulated as:

% \begin{equation}
\begin{gather}
\mathbf{Q} = \mathbf{X} \mathbf{W}^{\top}_\mathrm{q}, \quad 
\mathbf{K} = \mathbf{X} \mathbf{W}^{\top}_\mathrm{k}, \quad 
\mathbf{V} = \mathbf{X} \mathbf{W}^{\top}_\mathrm{v} \\
\operatorname{Attention-Out}
= \left[ \operatorname{softmax}\left( \frac{\mathbf{Q} \mathbf{K}^{\top}}{\sqrt{d_k}} \right) \mathbf{V}\right] \mathbf{W}^{\top}_\mathrm{o}
\end{gather}
% \end{equation}

We prove the output consistency before and after the input channel permutation of $\mathbf{W}^{\top}_\mathrm{o}$ as follows:

\begin{equation}
\resizebox{0.48\textwidth}{!}{$
\begin{aligned}
\widehat{\operatorname{Attention-Out}} &= \left[ \operatorname{softmax}\left( \frac{(\mathbf{X}\mathbf{W}^{\top}_\mathrm{q}\mathbf{P}^{\top}_\text{in})(\mathbf{X}\mathbf{W}^{\top}_\mathrm{k}\mathbf{P}^{\top}_\text{in})^{\top}}{\sqrt{d_k}} \right)(\mathbf{X}\mathbf{W}^{\top}_\mathrm{v}\mathbf{P}^{\top}_\text{in}) \right](\mathbf{P}_\text{in}\mathbf{W}^{\top}_\mathrm{o}) \\
&=\operatorname{softmax}\left( \frac{\mathbf{X}\mathbf{W}^{\top}_\mathrm{q}\mathbf{P}^{\top}_\text{in}\mathbf{P}_\text{in}\mathbf{W}_\mathrm{k}\mathbf{X}^{\top}}{\sqrt{d_k}} \right)(\mathbf{X}\mathbf{W}^{\top}_\mathrm{v}\mathbf{P}^{\top}_\text{in}\mathbf{P}_\text{in}\mathbf{W}^{\top}_\mathrm{o}) \\
&=\operatorname{softmax}\left( \frac{\mathbf{X}\mathbf{W}^{\top}_\mathrm{q}\mathbf{W}_\mathrm{k}\mathbf{X}^{\top}}{\sqrt{d_k}} \right)(\mathbf{X}\mathbf{W}^{\top}_\mathrm{v}\mathbf{W}^{\top}_\mathrm{o}) \\
&=\left[ \operatorname{softmax}\left( \frac{\mathbf{Q} \mathbf{K}^{\top}}{\sqrt{d_k}} \right) \mathbf{V}\right] \mathbf{W}^{\top}_\mathrm{o} \\
&=\operatorname{Attention-Out}
\end{aligned}$}
\end{equation}

Similarly, the permutation of the input channel for \(\mathbf{W}^{\top}_\mathrm{q}, \mathbf{W}^{\top}_\mathrm{k}, \mathbf{W}^{\top}_\mathrm{v} \) requires implementation of the corresponding output channel permutation for the previous layer. The FFN submodule typically consists of two parallel expansion matrices \(\mathbf{W}^{\top}_{\mathrm{up}}, \mathbf{W}^{\top}_{\mathrm{gate}} \in \mathbb{R}^{d_{\text{hidden}} \times d_{\text{ff}}}\) followed by a down-projection \(\mathbf{W}^{\top}_{\mathrm{down}} \in \mathbb{R}^{d_{\text{ff}} \times d_{\text{hidden}}}\). The two expansion paths operate on the same input and their outputs are combined multiplicatively. Therefore, the input channel permutation matrix \(\mathbf{P}_{\text{in}}\in\mathbb{R}^{d_{\text{ff}}\times d_{\text{ff}}}\) for \( \mathbf{W}^{\top}_\mathrm{down} \) should be applied identically to the others' output channels:

\begin{equation}
\resizebox{0.43\textwidth}{!}{$
\begin{aligned}
\widehat{\mathbf{W}}_{\mathrm{up}} =  \mathbf{W}^{\top}_{\mathrm{up}}\mathbf{P}^{\top}_{\text{in}},
\widehat{\mathbf{W}}_{\mathrm{gate}} =  \mathbf{W}^{\top}_{\mathrm{gate}}\mathbf{P}^{\top}_{\text{in}},
\widehat{\mathbf{W}}_{\mathrm{down}} =  \mathbf{P}_{\text{in}}\mathbf{W}^{\top}_{\mathrm{down}}.
\end{aligned}$}
\label{eq:4}
\end{equation}

Given the standard FFN computation formulated as:

\begin{equation}
\operatorname{FFN-Out} = \left[\texttt{act}(\mathbf{X}\mathbf{W}^{\top}_\mathrm{gate}) \otimes(\mathbf{X}\mathbf{W}^{\top}_\mathrm{up})\right]\mathbf{W}^{\top}_\mathrm{down}
\end{equation}

We prove the output consistency before and after the input channel permutation of $\mathbf{W}^{\top}_\mathrm{down}$ as follows:

\begin{equation}
\resizebox{0.48\textwidth}{!}{$
\begin{aligned}
\widehat{\operatorname{FFN-Out}} &= \left[\texttt{act}(\mathbf{X}\mathbf{W}^{\top}_\mathrm{gate}\mathbf{P}^{\top}_\text{in}) \otimes(\mathbf{X}\mathbf{W}^{\top}_\mathrm{up}\mathbf{P}^{\top}_\text{in})\right]\mathbf{P}_\text{in}\mathbf{W}^{\top}_\mathrm{down} \\
&= \left[\texttt{act}(\mathbf{X}\mathbf{W}^{\top}_\mathrm{gate})\mathbf{P}^{\top}_\text{in} \otimes(\mathbf{X}\mathbf{W}^{\top}_\mathrm{up})\mathbf{P}^{\top}_\text{in}\right]\mathbf{P}_\text{in}\mathbf{W}^{\top}_\mathrm{down} \\
&= \left[\texttt{act}(\mathbf{X}\mathbf{W}^{\top}_\mathrm{gate}) \otimes(\mathbf{X}\mathbf{W}^{\top}_\mathrm{up})\right]\mathbf{P}^{\top}_\text{in}\mathbf{P}_\text{in}\mathbf{W}^{\top}_\mathrm{down} \\
&= \left[\texttt{act}(\mathbf{X}\mathbf{W}^{\top}_\mathrm{gate}) \otimes(\mathbf{X}\mathbf{W}^{\top}_\mathrm{up})\right]\mathbf{W}^{\top}_\mathrm{down} \\
&=\operatorname{FFN-Out}
\end{aligned}$}
\end{equation}

In this case, the computational logics of elementwise-based \texttt{act} operation and channel permutation operation are independent of each other, allowing the existence of exchange laws for both.

Building upon the proven invariance of Transformer layers under permutation, these constraints necessitate that channel permutations be applied not independently, but jointly via coupled operations. This structured approach enforces shared permutations and inverse propagation within blocks, ensuring permutation-aware sparsification preserves functional dependencies, semantic integrity, and compatibility with structured compression techniques.

\begin{table*}[t]
\centering
\resizebox{\textwidth}{!}{
\begin{tabular}{c|l|c|ccccccc|c}
\toprule
\textbf{Model} & \multicolumn{1}{c|}{\textbf{Method}} & \textbf{Wikitext2} & \textbf{Arc-Easy} & \textbf{Arc-Challenge} & \textbf{BoolQ} & \textbf{HellaSwag} & \textbf{OpenBookQA} & \textbf{WinoGrande} & \textbf{MMLU} & \textbf{Average} \\ \midrule
\multirow{8}{*}{\shortstack[c]{LLaMA‑2‑7B\\(4:8)}}
 & Dense & 5.12 & 76.30 & 43.43 & 77.68 & 57.14 & 31.40 & 69.06 & 45.84 & 57.96 \\ \cmidrule{2-11}
 & Magnitude & 16.23 & 64.69 & 35.92 & 62.63 & 50.08 & 26.00 & 62.27 & 28.07 & 47.09 \\
 & SparseGPT & 7.84 & 69.61 & 36.77 & 72.11 & 48.27 & 27.40 & 68.35 & 32.81 & 50.76 \\
 & Wanda & 8.07 & 67.26 & 34.30 & 73.91 & 46.95 & 26.20 & 66.81 & 26.11 & 48.76 \\
 & PrunerZero & 8.52 & 65.70 & 33.36 & 69.27 & 45.58 & 23.20 & 66.30 & 28.81 & 47.46 \\
 & Perm & 8.11 & 66.92 & 34.51 & 72.88 & 46.18 & 26.17 & 66.64 & 26.13 & 48.49 \\
 & RIA & 7.92 & 67.85 & 33.92 & 72.26 & 47.12 & 27.32 & 66.89 & 26.82 & 48.88 \\
 & \cellcolor{gray!20}Ours & \cellcolor{gray!20}7.61 & \cellcolor{gray!20}68.51 & \cellcolor{gray!20}35.02 & \cellcolor{gray!20}73.88 & \cellcolor{gray!20}47.63 & \cellcolor{gray!20}28.15 & \cellcolor{gray!20}66.73 & \cellcolor{gray!20}28.67 & \cellcolor{gray!20}49.80 \\
\bottomrule
\end{tabular}
}
\caption{Performance of different methods on LLaMA2-7B model after 4:8 structured pruning.}
\label{tab:llama7b48}
\end{table*}

\subsection{More Details of Differentiable Bipartite Matching Solver}
\label{sec:match}
To enable end-to-end optimization of the permutation, we design a differentiable bipartite matching solver that learns discrete permutation matrices in a gradient-friendly manner. The module begins with a learned cost matrix and applies Sinkhorn-based relaxation to approximate the optimal permutation in a differentiable form. During inference, it is converted into a discrete matrix using the Hungarian algorithm. In the following, we walk through each component of this solver, from group-wise matching to soft relaxation and final discretization.

As detailed in Algorithm~\ref{alg:matching}, the solver begins by converting the input cost matrix \(\mathbf{C}\) into a kernel matrix \(\mathbf{K}\) using an element-wise exponential scaling with temperature \(\varepsilon\). The algorithm then performs Sinkhorn iterations in the log domain to compute the scaling vectors \(u\) and \(v\), which normalize the rows and columns of \(\mathbf{K}\) to form a doubly stochastic matrix \(\mathbf{P}\). These steps (lines 3--10) produce a soft permutation that approximates a valid assignment while maintaining numerical stability and supporting gradient flow. After the iterations, the algorithm recovers the soft permutation by combining \(u\), \(\mathbf{K}\), \(v\), and rescaling (line 11, 12). Finally, to obtain a discrete permutation for inference, it applies the Hungarian algorithm to select the minimum-cost one-to-one assignment from the soft matrix \(\mathbf{P}\) (line 13), resulting in a binary permutation matrix \(\Pi\). The algorithm outputs both \(\mathbf{P}\) and \(\Pi\) for training and inference, respectively.

\begin{algorithm}[t]
\caption{Workflow of Differentiable Bipartite Matching Solver}
\label{alg:matching}
\begin{algorithmic}[1]
\STATE \textbf{Input:} Cost matrix $\mathbf{C} \in \mathbb{R}^{N \times N}$, temperature $\varepsilon > 0$, number of iterations $T$
\STATE \textbf{Output:} Soft permutation matrix $\mathbf{P}$, discrete permutation matrix $\Pi$

\STATE $\mathbf{K} \gets \exp(-\mathbf{C} / \varepsilon)$
\STATE $\log \mathbf{K} \gets \log(\mathbf{K})$
\STATE Initialize $\log u \gets \mathbf{0},\quad \log v \gets \mathbf{0}$

\FOR{$t = 1$ to $T$}
    \STATE $\log u \gets -\,\mathrm{logsumexp}(\log \mathbf{K} + \log v,\; \text{dim}=1)$
    \STATE $\log v \gets -\,\mathrm{logsumexp}(\log \mathbf{K}^{\top} + \log u,\; \text{dim}=1)$
\ENDFOR
\STATE $u \gets \exp(\log u),\quad v \gets \exp(\log v)$
%\STATE $\mathbf{P} \gets \mathrm{Diag}(u)\, \mathbf{K}\, \mathrm{Diag}(v)$
\STATE $ \mathbf{P} \leftarrow \text{Diag}(u) \cdot K \cdot \text{Diag}(v)$

\STATE $\mathbf{P} \gets P \times \text{Size}(C)[0]$

\STATE $\Pi \gets \arg\min_{\mathbf{P} \in \mathcal{P}} \langle \mathbf{C}, \mathbf{P} \rangle$ \COMMENT{Hungarian algorithm}
\STATE $\Pi_{i,j} \in \{0, 1\}$ (discrete one-to-one permutation)

\STATE \textbf{return} $\mathbf{P}$, $\mathbf{\Pi}$
\end{algorithmic}
\end{algorithm}

\subsection{Performance across More Sparsity Patterns}

We further evaluate the effectiveness of our learnable permutator under more  structured sparsity settings, specifically the 4:8 sparsity pattern on the \texttt{LLaMA2-7B} model. As shown in Table~\ref{tab:llama7b48}, our method achieves the highest average accuracy of 49.80\%, outperforming existing baselines including Wanda (48.76\%), CP (48.16\%), and RIA (48.88\%). Notably, our method maintains strong performance on both reasoning tasks such as \texttt{Arc-Challenge} and \texttt{BoolQ}, as well as on harder language modeling benchmarks such as \texttt{WikiText2}, where it significantly reduces perplexity. These results highlight the robustness of our learned permutation under less common sparsity configurations, further demonstrating its generalizability across structured pruning setups.
